# Supplementary material for: Transparency, Privacy, and Fairness in Recommender Systems
Source: arXiv:2406.11323 source file (2024-06-28)
Supplement: Supplementary file 1 [file own_publications.tex]

This chapter describes my own contributions to the 17 main publications of this cumulative habilitation. All of these publications were created in a joint effort with my co-authors, and I would like to thank them again here for the great collaborations that made these publications possible.

Furthermore, the habilitation guidelines of Graz University of Technology require that own contributions to papers with co-authors are highlighted. I do this in Table~\ref{tab:papers_own} by stating my contributions to the publications below each paper reference in the table. Wherever possible, the stated contributions are in line with the author contribution sections of the given journal papers.

\begin{longtable}{p{1cm} p{12cm}}
\caption{Description of own contributions to the main publications selected by the author of the habilitation. } \\ \hline

\textbf{No.} & \textbf{Publication}\\\hline\hline

& \textbf{Transparency and Cognitive Models in Recommender Systems}\\\hline

\idHCI & Seitlinger, P., Ley, T., \textbf{Kowald, D.}, Theiler, D., Hasani-Mavriqi, I., Dennerlein, S., Lex, E., Albert, D. (2018). Balancing the Fluency-Consistency Tradeoff in Collaborative Information Search with a Recommender Approach. 
\textit{International Journal of Human–Computer Interaction}, 34:6, pp. 557-575.   
DOI: \url{https://doi.org/10.1080/10447318.2017.1379240}\\\\

& I contributed to the research idea of this paper and developed large parts of the bookmarking interface, which was used to conduct the study. I also developed the tag recommendation algorithms (\textit{MostPopular} and \textit{SoMe}), integrated them into the bookmarking interface, as well as contributed to the technical user study setup, data collection procedure, and the evaluation of the recommendation results. Additionally, I contributed to writing the paper throughout all iterations of writing. Apart from that, I was the first author of a short version of this publication, which I presented in the poster track of TheWebConf'2018.\\\hline

\idTISMIR & Lex, E.*, \textbf{Kowald, D.*},  Schedl, M. (2020). Modeling Popularity and Temporal Drift of Music Genre Preferences. \textit{Transactions of the International Society for Music Information Retrieval}, 3:1, pp. 17-30. (*equal contribution) 
DOI: \url{https://doi.org/10.5334/tismir.39}\\\\

& I shared the first authorship of the paper with Elisabeth Lex. Together, we created the research idea, methodology, and main text of this paper. Apart from that, I created the Last.fm dataset sample used in the paper, identified the different user groups in the dataset, developed the cognitive-inspired recommendation algorithms, and evaluated them using the \emph{TagRec} framework, for which I am the main developer. I also created all tables and figures presented in the paper.\\\hline

\idIUI & \textbf{Kowald, D.*}, Lex, E.*, Schedl, M. (2020). Utilizing Human Memory Processes to Model Genre Preferences for Personalized Music Recommendations. In \textit{4th Workshop on Transparency and Explainability in Adaptive Systems through User Modeling Grounded in Psychological Theory (HUMANIZE @ ACM IUI'2020)}. (*equal contribution) DOI: \url{https://doi.org/10.48550/arXiv.2003.10699}\\\\

& As in the case of~\idTISMIR, I shared the first authorship of this paper with Elisabeth Lex, and together, we created the research idea, methodology, and main text of the paper. In addition, I developed and evaluated the semantic context component of the activation equation of the cognitive model ACT-R, and integrated it into the \emph{TagRec} framework. I discussed the difference between the full activation equation and base-level learning equation of ACT-R, and created all tables and figures.\\\hline

\idFNT & Lex, E., \textbf{Kowald, D.}, Seitlinger, P., Tran, T., Felfernig, A., Schedl, M. (2021). Psychology-informed Recommender Systems. \textit{Foundations and Trends in Information Retrieval}, 15:2, pp. 134–242. 
DOI: \url{https://doi.org/10.1561/1500000090}\\\\

& I contributed to the general idea and the survey method of this paper. I also contributed to the sections on cognitive-inspired recommender systems and cognitive models of attention, to all discussion subsections in the paper, the formalization of activation process in human memory, and created the schematic illustration of the ACT-R architecture. Finally, I contributed to writing the paper throughout all iterations of writing, and supported in identifying potential avenues for future research, as well as discussing how cognitive models contribute to transparency aspects.\\\hline

\idRecSysACTR & Moscati, M., Wallmann, C., Reiter-Haas, M., \textbf{Kowald, D.}, Lex, E., Schedl, M. (2023). Integrating the ACT-R Framework and Collaborative Filtering for Explainable Sequential Music Recommendation.  In \textit{Proceedings of the 17th ACM Conference on Recommender Systems (RecSys'2023)}, pp. 840–847. 
DOI: \url{https://doi.org/10.1145/3604915.3608838}\\\\

& I contributed to the description of the method and experimental setup, and to the description and interpretation of the results, as well as to paper writing during all iterations. Specifically, I contributed to formalizing the components of the recommendation approach based on ACT-R, and to interpreting the weights of the ACT-R components towards providing transparent and explainable recommendations.\\\hline\hline

& \textbf{Privacy and Limited Preference Information in Recommender Systems}\\\hline

\idRecSysTRUST & Duricic, T., Lacic, E., \textbf{Kowald, D.}, Lex, E. (2018). Trust-Based Collaborative Filtering: Tackling the Cold Start Problem Using Regular Equivalence. In \textit{Proceedings of the 12th ACM Conference on Recommender Systems (RecSys'2018)}, pp. 446–450. 
DOI: \url{https://doi.org/10.1145/3240323.3240404}\\\\

& I contributed to formalizing the approach based on Katz similarity, and defining the user cold-start experimental setup used to evaluate the trust-based recommendations. Additionally, I was involved in the interpretation of the evaluation results, and all iterations of paper writing. This paper is part of Tomislav Duricic's (first author) ongoing Ph.D. thesis, for which I am co-supervisor together with Elisabeth Lex.\\\hline

\idUMUAI & Lacic, E., Reiter-Haas, M., \textbf{Kowald, D.}, Dareddy, M., Cho, J., Lex, E. (2020). Using Autoencoders for Session-based Job Recommendations. \textit{User Modeling and User-Adapted Interaction}, 30, pp. 617–658. 
DOI: \url{https://doi.org/10.1007/s11257-020-09269-1}\\\\

& I contributed to empirical research, the experimental setup, description of the session-based recommendation approach based on limited preference information of the users, definition of the autoencoder-based system architecture, interpretation and discussion of results, and paper writing in all iterations. Specifically, I contributed to the formal definition and implementation of the beyond-accuracy metrics system-based novelty and session-based novelty.\\\hline

\idEcirMETA & Muellner, P., \textbf{Kowald, D.}, Lex, E. (2021). Robustness of Meta Matrix Factorization Against Strict Privacy Constraints. In \textit{Proceedings of the 43rd European Conference on Information Retrieval (ECIR'2021)}, pp. 107-119. 
DOI: \url{https://doi.org/10.1007/978-3-030-72240-1_8}\\\\

& I contributed to the original research idea of this paper, to the methodology of the reproducibility and privacy-focused studies, description and interpretation of the results, and paper writing in all iterations. I especially supported in defining the experiments to study the users' privacy constraints. This paper is part of Peter Muellner's (first author) ongoing Ph.D. thesis, for which I am co-supervisor together with  Elisabeth Lex. Apart from that, I was the last author of a short version of this publication, which was presented at the Responsible AI Forum 2021.\\\hline 

\idTIST & Muellner P., Lex, E., Schedl, M., \textbf{Kowald, D.} (2023). ReuseKNN: Neighborhood Reuse for Differentially-Private KNN-Based Recommendations. \textit{ACM Transactions on Intelligent Systems and Technology}, 14:5, pp. 1-29. 
DOI: \url{https://doi.org/10.1145/3608481}\\\\

& As last author, I contributed to the original research idea, finding and describing related work, defining the problem setting, formalizing the approach and the evaluation settings, and interpreting the evaluation results. I also contributed to discussing the trade-off between privacy and accuracy. Additionally, I contributed to paper writing in all iterations. This paper is part of Peter Muellner's (first author) ongoing Ph.D. thesis, for which I am co-supervisor together with Elisabeth Lex.\\\hline

\idFRONTPRI & Muellner P., Lex, E., Schedl, M., \textbf{Kowald, D.} (2023). Differential Privacy in Collaborative Filtering Recommender Systems: A Review.  \textit{Frontiers in Big Data}, 6:1249997, pp. 1-7. 
DOI: \url{https://doi.org/10.3389/fdata.2023.1249997}\\\\

& As last and corresponding author of this article, I contributed to the original idea, conceptualization, writing process throughout all iterations, and supervision of the review methodology and the paper writing process. Additionally, I contributed to the categorization of the 26 publications reviewed in this article, and to the identification of open research questions in the field of differentially private recommender systems. This article is part of Peter Muellner's (first author) ongoing Ph.D. thesis, for which I am co-supervisor together with Elisabeth Lex.\\\hline\hline

& \textbf{Fairness and Popularity Bias in Recommender Systems}\\\hline

\idEcirPOP & \textbf{Kowald, D.}, Schedl, M., Lex, E. (2020). The Unfairness of Popularity Bias in Music Recommendation: A Reproducibility Study. In \textit{Proceedings of the 42nd European Conference on Information Retrieval (ECIR'2020)}, pp. 35-42. 
DOI: \url{https://doi.org/10.1007/978-3-030-45442-5_5}\\\\

& As first and corresponding author of this paper, I contributed to the research idea, created the first full draft of the paper, created the Last.fm dataset sample, implemented the recommendation algorithms and evaluation methods, conducted the experiments, and described and interpreted the results. The source-code for this publication started my \emph{FairRecSys} \textit{GitHub} repository, which contains Python scripts for studying fairness and popularity bias in recommender systems. I also presented the paper in the reproducibility track of the \textit{European Conference on Information Retrieval (ECIR'2020)}.\\\hline

\idEPJ & \textbf{Kowald, D.}, Muellner, P., Zangerle, E., Bauer, C., Schedl, M., Lex, E. (2021). Support the Underground: Characteristics of Beyond-Mainstream Music Listeners. \textit{EPJ Data Science}, 10:14. 
DOI: \url{https://doi.org/10.1140/epjds/s13688-021-00268-9}\\\\

& As first and corresponding author of this publication, I contributed to the original idea, the collection of related work, identification of beyond-mainstream users in the Last.fm dataset, data analysis methods, and description and interpretation of results, as well as large parts of the paper writing process during all iterations. I also contributed to establish the connection between the recommendation accuracy results of the subgroups and openness patterns of these subgroups. This paper was part of Peter Muellner's (second author) Master's thesis, for which I was co-supervisor together with Elisabeth Lex. I was also involved in interviews discussing the findings of this paper for several news outlets (e.g., Rolling Stone Italy or BioMed Central).\\\hline

\idRecSysLBR & Lesota, O., Melchiorre, A., Rekabsaz, N., Brandl, S., \textbf{Kowald, D.}, Lex, E., Schedl, M. (2021). Analyzing Item Popularity Bias of Music Recommender Systems: Are Different Genders Equally Affected? In \textit{Proceedings of the 15th ACM Conference on Recommender Systems (RecSys'2021)}, pp. 601-606. 
DOI: \url{https://doi.org/10.1145/3460231.3478843}\\\\

& I contributed to the conceptualization, finding and description of related work, methodology for measuring popularity bias across genders, investigation and interpretation of the results, and paper writing in all iterations. Specifically, I contributed to defining delta metrics for measuring popularity bias based on the delta group average popularity metric, which was proposed for music recommendations in~\idEcirPOP.\\\hline 

\idBiasMEDIA & \textbf{Kowald, D.}, Lacic, E. (2022). Popularity Bias in Collaborative Filtering-Based Multimedia Recommender Systems. In \textit{Advances in Bias and Fairness in Information Retrieval (BIAS @ ECIR'2022)}. Communications in Computer and Information Science, vol. 1610, pp. 1-11. 
DOI: \url{https://doi.org/10.1007/978-3-031-09316-6_1}\\\\

& As first and corresponding author of this paper, I contributed to the research idea, created the first full draft of the paper, created the dataset samples and user group divisions, implemented the recommendation algorithms and evaluation methods using my \emph{FairRecSys} \textit{GitHub} repository, conducted the experiments, and described and interpreted the results. I also presented the paper at the \textit{European Conference on Information Retrieval (ECIR'2022)}. Together with Emanuel Lacic, I was awarded with the \textit{Mind-the-Gap Gender and Diversity} award of Graz University of Technology for this paper.\\\hline

\idEcirPRESSE & Lacic, E., Fadljevic, L., Weissenboeck, F., Lindstaedt, S., \textbf{Kowald, D.} (2022). What Drives Readership? An Online Study on User Interface Types and Popularity Bias Mitigation in News Article Recommendations. In \textit{Proceedings of the 44th European Conference on Information Retrieval (ECIR'2022)}, pp. 172-179. 
DOI: \url{https://doi.org/10.1007/978-3-030-99739-7_20}\\\\

& As last and corresponding author of this paper, I contributed to the original research idea, the design of the content-based news article recommendation algorithm, the definition of the research questions and experimental setup, the design of the online user study, the choice of suitable evaluation metrics, and the description and interpretation of the results. I did the main communications with representatives of the news platform \textit{DiePresse}, and  created a first full draft of the paper together with the first author, Emanuel Lacic. Together, we presented the paper at the \textit{European Conference on Information Retrieval (ECIR'2022)}.\\\hline 

\idBiasCALIBRATION & \textbf{Kowald, D.*}, Mayr, G.*, Schedl, M., Lex, E. (2023). A Study on Accuracy, Miscalibration, and Popularity Bias in Recommendations. In \textit{Advances in Bias and Fairness in Information Retrieval (BIAS @ ECIR'2023)}. Communications in Computer and Information Science, vol. 1840, pp. 1-16. (*equal contribution) 
DOI: \url{https://doi.org/10.1007/978-3-031-37249-0_1}\\\\

& As first and corresponding author of this publication, I contributed to the original idea, the methodology, the creation of the dataset samples, interpretation of results, and paper writing in all iterations. Specifically, I extracted the genre information of the three datasets, and assigned the genres to the corresponding items using my \emph{FairRecSys} \textit{GitHub} repository. This paper was part of Gregor Mayr's (co-first author) Bachelor's thesis and Master's project, for which I was co-supervisor together with Elisabeth Lex. I also presented the paper at the \textit{European Conference on Information Retrieval (ECIR'2023)}.\\\hline

\idSCIREP & Scher, S., Kopeinik, S., Truegler, A., \textbf{Kowald, D.} (2023). Long-Term Dynamics of Fairness: Understanding the Impact of Data-Driven Targeted Help on Job Seekers. \textit{Nature Scientific Reports}, 13:1727.  
DOI: \url{https://doi.org/10.1038/s41598-023-28874-9}\\\\

& As last author, I contributed to the analysis of the data, the discussion and interpretation of the empirical results, and writing of the manuscript in all iterations of the writing process. Additionally, I contributed to formalizing and describing the trade-off between the different long-term fairness goals, and to relating them to the trade-off between individual and group fairness. Together with the first two authors of this publication, I set up Master thesis topics to transfer the methodology of this study to the area of fair recommender systems.\\\hline 

\label{tab:papers_own}
\end{longtable}

As described in this table, I contributed substantially to all 17 publications, and for 10 of these publications I am also either first or last author. In the following, the full texts of the papers are given. I use the published journal and conference formats for all papers, except for~\idFNT, where I altered the formatting slightly due to copyright restrictions of the journal's publisher.
